# Supplementary material for: Piezoplasmonics: strain-induced tunability of plasmon resonance in AlAs quantum wells
Source: arXiv:2011.09139 source file (2020-11-18)
Supplement: Supplementary file 1 [file Supplementary.pdf]

# Supplementary Material for
# "Piezoplasmonics: Giant stress-induced tunability of plasmon resonance in AlAs quantum wells"

A. R. Khisameeva, V. M. Muravev, I. V. Kukushkin
*Institute of Solid State Physics, RAS, Chernogolovka, 142432 Russia*
(Dated: November 18, 2020)

## I. PIEZO-STACK CALIBRATION

In our experiments, we used a ceramic piezo-stack actuator (PSA) with semi-bipolar operation (PSt 150hTc/5x5/7). The sample was glued on the top surface of PSA with [010] crystallographic direction aligned along the stroke direction. A positive voltage on PSA stretched the sample along the poling direction and shrank in the transverse direction.

To calibrate the strain applied to the sample, we used a bridge scheme (Fig. 1(a)), in which the resistive strain gauge (foil strain gauge 1-LY1x-3/120 from Hottinger Baldwin Measurements, Inc.) was glued to the backside of the PSA. The bridge circuit consists of two resistors $R_2$, $R_4$ and two strain gauges $R_1$, $R_3$ all with equal resistance values of $120\,\Omega$. One of the SG was glued on the piezo-stack to measure applied deformation (active). The second gauge (dummy) worked as a compensation element to eliminate the influence of the temperature change. It was not subject to a mechanical strain. We applied a voltage $V_{\mathrm{in}}$ to the bridge and measured the voltage $V_{\mathrm{out}}$ across the bridge branches (Fig. 1(a)). We used a lock-in technique to reduce the noises. Assuming that $R_1 = R_2 = R_3 = R_4 = R$, we arrive at

$$\frac{V_{\mathrm{out}}}{V_{\mathrm{in}}} = \frac{\Delta R_1}{4R}, \tag{S1}$$

where $\Delta R_1$ is a resistance change due to the deformation. The mechanical strain $\varepsilon = \dfrac{\Delta L}{L} = \dfrac{\Delta R}{R}\dfrac{1}{k}$, where $\Delta L$ is the absolute change in length, $L$ is the original length, $k$ is the gauge factor. According to the documentation $k = 2$. The applied deformation then reads

$$\varepsilon = \frac{2\Delta V_{\mathrm{out}}}{V_{\mathrm{in}}} \tag{S2}$$

The resulting dependency of deformation $\varepsilon$ on applied bias voltage to the piezo-stack $V_{\mathrm{p}}$ is shown in Fig. S1(b). The dependence is linear. The measurements were carried out at a temperature of $T = 4.2$ K.

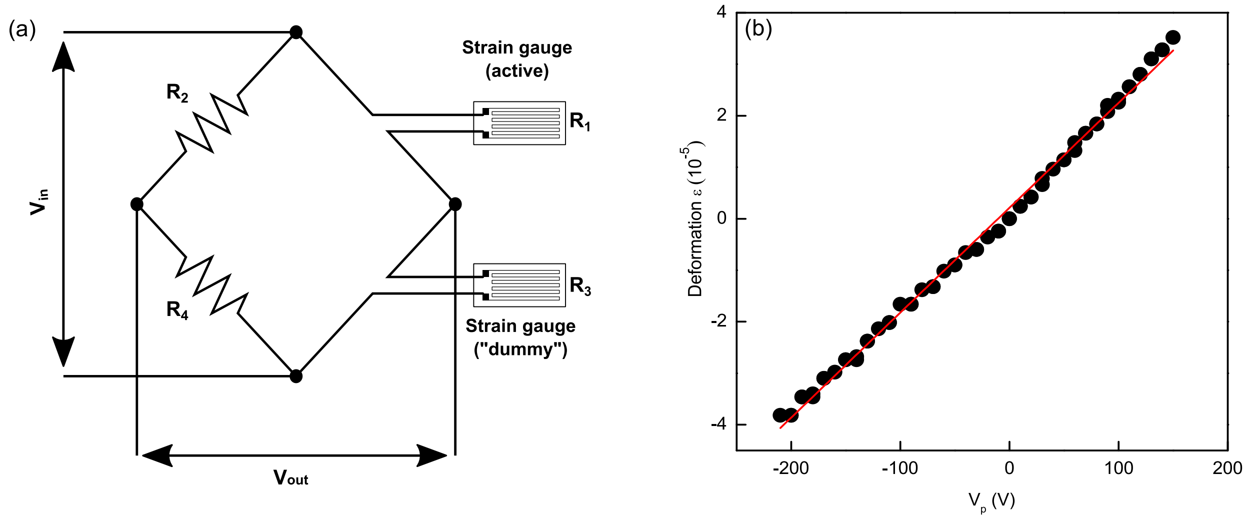


FIG. S1: (a) Schematic drawing of measuring quarter-bridge circuit. (b) Deformation $\varepsilon$ of the sample vs. applied bias voltage (at T = 4.2 K) is measured using a strain gauge (SG) glued on the piezo-stack.

## II. ANALYSIS OF THE RESONANCE LINESHAPE AND POSITION

The typical lineshape of resonance is shown in Fig. S2. It consists of constant background and negative part related to the absorption of the incident microwave radiation inside AlAs disks, $T(B) = \text{const} - T_{\text{abs}}(B)$. In the linear response regime, the absorption is proportional to the real part of the conductivity, $T_{\text{abs}} \propto \text{Re}\,\sigma$. The exact expression depends on the geometry.

For the linear polarized microwave radiation the real part of the conductivity can be approximated by the Drude formula:

$$\text{Re}\,\sigma_{xx} = \frac{\sigma_0}{2\tau^2}\left(\frac{1}{(\omega-\omega_c)^2+1/\tau^2}+\frac{1}{(\omega+\omega_c)^2+1/\tau^2}\right), \quad \sigma_0 = \frac{ne^2\tau}{m}, \quad \omega_c = \frac{eB}{\sqrt{m_l m_{\text{tr}}}}.$$

Therefore, the absorption can be expressed as

$$T_{\text{abs}}(B) = T_0\left[\frac{1}{1+(2(B-B_0)/\Gamma)^2}+\frac{1}{1+(2(B+B_0)/\Gamma)^2}\right]. \tag{S3}$$

Here, $B_0$ is the magnetic-field position of the resonance, $\Gamma$ and $T_0$ denotes the width and amplitude of the resonance, respectively. The typical fits are shown in Fig. S2 by red curves.

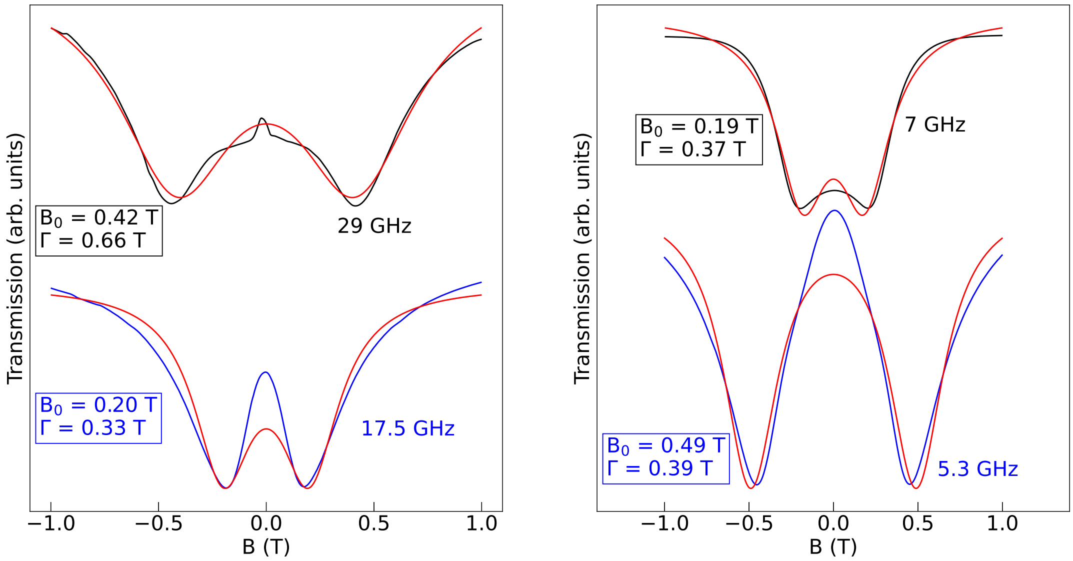


FIG. S2: Resonance fitting for CPW magnetic field transmission curves of the two-dimensional plasma excitations in AlAs disks for the sample without external deformation ($n_s = 2.4 \times 10^{11}$ cm$^{-2}$): (a) cyclotron magnetoplasma mode at $f = 17.5$ and 23.5 GHz; (b) EMP mode at $f = 7$ and 5.3 GHz. Red lines represent fitting using Eq. (S3), while black lines correspond to experimental data.

## III. MAGNETODISPERSION OF PLASMA RESONANCE FOR ANISOTROPIC 2DES

Analytical derivation of plasmon magnetodispersion for quantum well with anisotropic effective masses in a disk geometry is a non-trivial task. It can be done in a dipole approximation when higher harmonics are neglected. The problem is then effectively equivalent to the motion of a single electron in a harmonic confining potential [1]. In this case, the Hamiltonian in the presence of the perpendicular magnetic field reads:

$$H = \frac{\left(\vec{p} - \frac{e}{c}\vec{A}\right)^2}{2m_c} + \frac{m_c}{2}(\Omega_{[100]}^2 x^2 + \Omega_{[010]}^2 y^2), \quad \vec{A} = \begin{pmatrix} -By \\ 0 \end{pmatrix}, \tag{S4}$$

where $m_c = \sqrt{m_\mathrm{l} m_\mathrm{t}}$ is electronic cyclotron mass, and $\Omega_{[100]}$ and $\Omega_{[010]}$ are plasma frequencies along the main crystallographic directions at $B = 0$ T. This approach is sometimes referred to as an elliptic model. It stems from the fact that results of the dipole approximation are equivalent to an exact solution for the lowest eigenmodes of the oblate spheroid with vanishing thickness.

Under the assumption of negligibly small retardation and dissipation $\omega_\mathrm{c}, \Omega_{[100],[010]} \gg \tau^{-1}$ ($\tau$ is the relaxation time of electrons, and $\omega_c = eB/m_c$ is the cyclotron frequency), the dipole approximation leads to the final expression of magnetodispersion for 2DES with a strong anisotropy of effective masses [2]:

$$\omega_\pm = \frac{1}{2}\left[\sqrt{(\Omega_{[100]} + \Omega_{[010]})^2 + \omega_c^2} \pm \sqrt{(\Omega_{[100]} - \Omega_{[010]})^2 + \omega_c^2}\right], \tag{S5}$$

In turn, the plasma frequencies $\Omega_{[100],[010]}$ are determined as [3]:

$$\Omega_{[100]}^2 = \frac{e^2 q}{2\kappa_0 \kappa^*}\left(\frac{n_\mathrm{x}}{m_\mathrm{l}} + \frac{n_\mathrm{y}}{m_\mathrm{tr}}\right), \tag{S6}$$

$$\Omega_{[010]}^2 = \frac{e^2 q}{2\kappa_0 \kappa^*}\left(\frac{n_\mathrm{x}}{m_\mathrm{tr}} + \frac{n_\mathrm{y}}{m_\mathrm{l}}\right). \tag{S7}$$

Here $\kappa^* = (\kappa_\mathrm{GaAs} + 1)/2$ is the effective dielectric permittivity of the surrounding medium and $q = 2.4/d$ is the wave vector in the disk geometry [4].

[1] C. Dahl, F. Brinkop, A. Wixforth, J. P. Kotthaus, J. H. English, and M. Sundaram, Solid State Commun. **80**, 673 (1991).
[2] V. A. Geyler, V. A. Margulis, and A. V. Shorokhov, Phys. Rev. B **63**, 245316 (2001).
[3] R. Z. Vitlina and A. V. Chaplik, Zh. Eksp. Teor. Fiz. **81**, 1011 (1981) [Sov. Phys. JETP **54**, 536 (1981)].
[4] I. V. Kukushkin, J. H. Smet, S. A. Mikhailov, D. V. Kulakovskii, K. von Klitzing, and W. Wegscheider, Phys. Rev. Lett. **90**, 156801 (2003).
